# Supplementary material for: Linear-scaling generation of potential energy surfaces using a double incremental expansion
Source: arXiv:1605.01674 ancillary file (2016-08-12)
Supplement: Supplementary file 1 [file supplementary_material.pdf]

– SUPPLEMENTARY MATERIAL –

# Linear-scaling generation of potential energy surfaces using a double incremental expansion

Carolin König[1, a)] and Ove Christiansen[1, b)]

*Department of Chemistry, Aarhus University, DK-8000 Aarhus C, Denmark.*

[a)] Electronic mail: carolink@kth.se

[b)] Electronic mail: ove@chem.au.dk

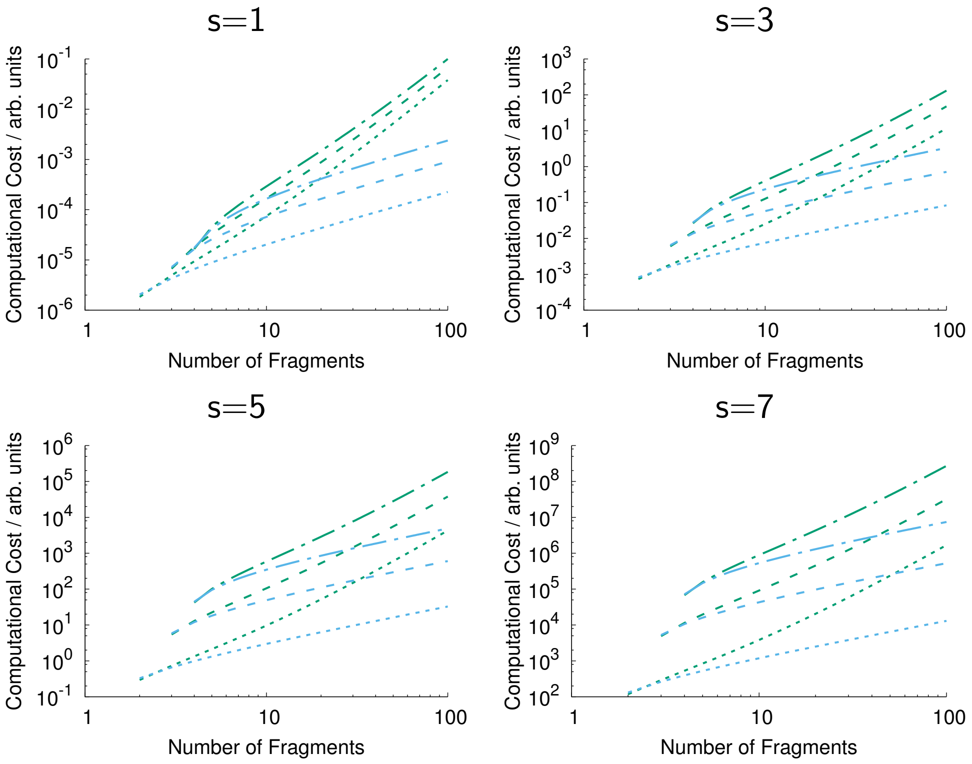


FIG. S-1. Estimated computational cost obtained by multiplying the number of SPCs for a certain system size of $l \cdot N_{\mathrm{pfr}}$ atoms by $A \cdot (l \cdot N_{\mathrm{pfr}})^s$, where $s = 1, 3, 5, 7$ and $A = 10^{-12}$ for the different schemes, i.e., DIF (green) and DIFACT (blue), different number of fragments ($F = 1 - 100$), and different fragment-combination level, i.e., $f = 2$ (- - -), $f = 3$ (——), and $f = 4$ (· — ·), distinguished by the line type. The values for the other parameters in Eqs. (40) and (41) in the main text are $N_{\mathrm{pfr}} = 10$, $n = 2$, and $g = 8$.

TABLE S-I. Applied bond length for capping of dangling bonds.

| Type | Length / Å | Classification in Ref. 1 |
|---|---|---|
| C–H | 1.059 | C-C-$H_3$ (methyl) |
| N–H | 1.009 | $X_2$–N-H |
| O–H | 0.967 | in alcohols C*–O–H |

[1] F. H. Allen, O. Kennard, D. G. Watson, L. Brammer, A. G. Orpen, and R. Taylor, J. Chem. Soc., Perkin Trans. 2 , S1 (1987).

TABLE S-II. Fundamental excitation energies from state-specific VSCF calculations for hexaphenyl considering only inter-connecting modes for the different approximations of the potential energy surfaces (all HF-3c). $\omega$ are the corresponding quasi-harmonic FALCON frequencies. All energies are given in $cm^{-1}$. The type label IC1 refers to [C1-B1]-(A1)↔(A2)-[B2-C2] type, IC2 to [C1]-(B1)↔(A1-A2)↔(B2)-[C2] type, and IC3 to (C1)↔(B1-A1-A2-B2)↔(C2) type of coordinates (see main text for further explanation).

| | Type | $\omega$ | 2M | DIF-$f$F2M | | | DIFACT-$f$F2M | | |
|---|---|---|---|---|---|---|---|---|---|
| $f$ | | | | 2 | 3 | 4 | 2 | 3 | 4 |
| 1 | IC3 | 41.24 | 51.52 | 51.57 | 51.52 | 51.52 | 52.43 | 51.51 | 51.04 |
| 2 | IC3 | 56.88 | 67.32 | 67.50 | 67.32 | 67.32 | 68.35 | 67.54 | 67.53 |
| 3 | IC3 | 59.18 | 89.11 | 89.31 | 89.14 | 89.12 | 87.49 | 91.23 | 91.93 |
| 4 | IC3 | 72.55 | 96.30 | 96.69 | 96.33 | 96.31 | 95.88 | 95.94 | 94.56 |
| 5 | IC3 | 73.99 | 80.87 | 80.65 | 80.87 | 80.87 | 81.17 | 80.67 | 80.53 |
| 6 | IC2 | 83.90 | 101.05 | 101.71 | 101.09 | 101.05 | 103.84 | 104.01 | 100.58 |
| 7 | IC2 | 93.37 | 108.43 | 109.08 | 108.44 | 108.42 | 110.11 | 106.01 | 108.16 |
| 8 | IC3 | 98.34 | 104.90 | 104.57 | 104.89 | 104.90 | 104.87 | 104.81 | 105.04 |
| 9 | IC1 | 102.13 | 115.44 | 116.15 | 115.47 | 115.44 | 116.31 | 115.15 | 115.77 |
| 10 | IC2 | 202.87 | 203.12 | 205.23 | 203.12 | 203.12 | 206.67 | 204.30 | 203.60 |
| 11 | IC2 | 216.07 | 217.49 | 219.54 | 217.51 | 217.49 | 220.55 | 217.52 | 217.48 |
| 12 | IC2 | 288.27 | 289.32 | 288.56 | 289.29 | 289.32 | 288.88 | 289.55 | 289.10 |
| 13 | IC2 | 297.93 | 297.57 | 296.86 | 297.55 | 297.57 | 298.00 | 298.51 | 298.03 |
| 14 | IC1 | 326.16 | 328.49 | 328.86 | 328.47 | 328.49 | 328.88 | 328.59 | 328.62 |
| 15 | IC3 | 335.64 | 339.42 | 339.64 | 339.44 | 339.42 | 339.49 | 338.61 | 338.89 |
| 16 | IC3 | 361.69 | 364.60 | 365.05 | 364.62 | 364.60 | 365.15 | 364.11 | 364.43 |
| 17 | IC1 | 370.76 | 372.24 | 371.21 | 372.17 | 372.23 | 370.82 | 372.16 | 372.32 |
| 18 | IC3 | 376.68 | 374.60 | 374.39 | 374.59 | 374.60 | 374.49 | 374.66 | 374.60 |
| 19 | IC3 | 404.40 | 405.70 | 405.37 | 405.68 | 405.69 | 405.51 | 405.35 | 405.40 |
| 20 | IC2 | 434.15 | 435.44 | 434.62 | 435.44 | 435.44 | 435.02 | 435.54 | 435.58 |
| 21 | IC3 | 447.10 | 447.70 | 447.35 | 447.69 | 447.70 | 447.69 | 447.55 | 447.64 |
| 22 | IC2 | 454.34 | 455.22 | 455.08 | 455.26 | 455.22 | 455.66 | 455.64 | 455.24 |
| 23 | IC3 | 462.35 | 459.44 | 459.25 | 459.43 | 459.44 | 459.24 | 459.47 | 459.42 |
| 24 | IC2 | 483.41 | 484.12 | 483.91 | 484.09 | 484.12 | 483.40 | 483.96 | 484.26 |
| 25 | IC1 | 503.08 | 503.77 | 503.09 | 503.84 | 503.77 | 502.98 | 503.90 | 503.84 |
| 26 | IC2 | 525.04 | 525.13 | 524.76 | 525.12 | 525.13 | 524.68 | 525.33 | 525.13 |
| 27 | IC2 | 536.92 | 534.06 | 533.15 | 534.02 | 534.05 | 533.16 | 534.53 | 534.53 |
| 28 | IC1 | 549.34 | 549.37 | 549.07 | 549.33 | 549.37 | 548.84 | 549.29 | 549.40 |
| 29 | IC2 | 600.50 | 597.12 | 596.12 | 597.05 | 597.12 | 596.19 | 597.08 | 596.80 |
| 30 | IC1 | 658.30 | 654.47 | 652.89 | 654.34 | 654.46 | 652.91 | 654.06 | 654.49 |

TABLE S-III: Fundamental excitation energies from state-specific VSCF calculations for tetraphenyl for the different approximations of the potential energy surfaces (all HF-3c). $\omega$ are the corresponding quasi-harmonic FALCON frequencies. All energies are given in $cm^{-1}$. The type labels A1, A2, B1, and B2 refer to intra-fragment vibrations in the respective fragments (see Figure 3 in the main text), IC1 refers to [B1]-(A1)↔(A2)-[B2] and IC2 to (B1)↔(A1-A2)↔(B2) type of FALCON coordinates (see main text for further explanation).

| No | Type | $\omega$ | 2M | DIF-$f$F2M | | DIFACT-$f$F2M | |
|---|---|---|---|---|---|---|---|
| $f$ | | | | 2 | 3 | 2 | 3 |
| 1 | IC2 | 45.95 | 60.30 | 60.37 | 60.30 | 60.99 | 60.15 |
| 2 | IC2 | 59.23 | 100.95 | 100.97 | 100.95 | 102.38 | 105.74 |
| 3 | IC2 | 74.54 | 83.77 | 83.93 | 83.77 | 85.14 | 85.66 |
| 4 | IC2 | 83.84 | 117.28 | 117.43 | 117.28 | 117.42 | 113.57 |
| 5 | IC2 | 87.92 | 101.42 | 101.44 | 101.42 | 101.80 | 101.56 |
| 6 | IC1 | 102.51 | 128.76 | 129.06 | 128.78 | 130.85 | 129.17 |
| 7 | IC2 | 132.33 | 140.84 | 140.44 | 140.83 | 140.74 | 140.98 |
| 8 | IC1 | 326.79 | 327.88 | 328.36 | 327.89 | 328.37 | 328.01 |
| 9 | IC2 | 349.13 | 351.23 | 351.55 | 351.22 | 352.43 | 350.71 |
| 10 | IC1 | 370.57 | 372.35 | 371.94 | 372.33 | 370.82 | 372.42 |
| 11 | IC2 | 376.65 | 372.29 | 372.07 | 372.29 | 371.98 | 372.11 |
| 12 | IC2 | 401.39 | 401.34 | 402.53 | 401.39 | 403.46 | 401.35 |
| 13 | IC2 | 428.26 | 427.68 | 427.42 | 427.65 | 428.53 | 427.65 |
| 14 | B1 | 474.94 | 481.45 | 481.51 | 481.45 | 481.16 | 481.39 |
| 15 | B2 | 474.96 | 481.45 | 481.50 | 481.45 | 481.16 | 481.39 |
| 16 | A2 | 481.65 | 486.34 | 486.46 | 486.33 | 486.94 | 486.52 |
| 17 | A1 | 481.65 | 486.34 | 486.46 | 486.33 | 486.94 | 486.52 |
| 18 | IC2 | 499.72 | 497.88 | 497.62 | 497.88 | 498.33 | 497.68 |
| 19 | IC1 | 503.33 | 500.94 | 500.41 | 500.97 | 500.20 | 501.08 |
| 20 | IC2 | 534.47 | 528.83 | 528.49 | 528.80 | 528.32 | 528.64 |
| 21 | IC1 | 549.26 | 547.68 | 547.69 | 547.68 | 547.16 | 547.73 |
| 22 | B1 | 566.25 | 574.75 | 574.92 | 574.76 | 574.56 | 574.67 |
| 23 | B2 | 566.27 | 574.75 | 574.92 | 574.76 | 574.55 | 574.66 |
| 24 | A2 | 628.14 | 643.23 | 645.45 | 643.25 | 645.88 | 643.44 |
| 25 | A1 | 628.18 | 643.23 | 645.44 | 643.25 | 645.87 | 643.44 |
| 26 | IC1 | 658.01 | 650.87 | 649.50 | 650.82 | 649.38 | 650.86 |
| 27 | B2 | 702.97 | 702.47 | 702.49 | 702.47 | 702.36 | 702.41 |
| 28 | B1 | 702.97 | 702.47 | 702.49 | 702.47 | 702.36 | 702.41 |
| 29 | A2 | 719.93 | 717.14 | 717.08 | 717.14 | 717.17 | 717.17 |
| 30 | A1 | 719.94 | 717.14 | 717.08 | 717.14 | 717.17 | 717.17 |
| 31 | B1 | 782.60 | 781.92 | 781.98 | 781.92 | 781.78 | 781.88 |
| 32 | B2 | 782.61 | 781.92 | 781.98 | 781.92 | 781.78 | 781.88 |
| 33 | B1 | 838.67 | 856.43 | 856.62 | 856.44 | 856.11 | 856.36 |
| 34 | B2 | 838.71 | 856.42 | 856.60 | 856.42 | 856.09 | 856.34 |
| 35 | A2 | 859.84 | 857.23 | 857.09 | 857.21 | 857.17 | 857.24 |
| 36 | A1 | 859.84 | 857.23 | 857.09 | 857.21 | 857.17 | 857.24 |
| 37 | A2 | 884.65 | 880.01 | 879.33 | 880.02 | 879.61 | 880.14 |
| 38 | A1 | 884.66 | 880.01 | 879.33 | 880.01 | 879.61 | 880.14 |
| 39 | B1 | 913.87 | 937.18 | 937.25 | 937.18 | 936.70 | 937.08 |
| 40 | B2 | 913.94 | 937.19 | 937.26 | 937.20 | 936.71 | 937.09 |
| 41 | A2 | 1019.93 | 1044.34 | 1045.30 | 1044.35 | 1045.83 | 1044.60 |
| 42 | A1 | 1019.98 | 1044.34 | 1045.30 | 1044.35 | 1045.83 | 1044.60 |
| 43 | A2 | 1033.14 | 1062.06 | 1062.49 | 1062.08 | 1063.05 | 1062.35 |
| 44 | A1 | 1033.19 | 1062.06 | 1062.49 | 1062.08 | 1063.05 | 1062.35 |
| 45 | B1 | 1037.13 | 1067.60 | 1067.86 | 1067.61 | 1067.47 | 1067.45 |

TABLE S-III continued: Fundamental excitation energies from state-specific VSCF calculations for tetra-phenyl for the different approximations of the potential energy surfaces (all HF-3c). $\omega$ are the corresponding quasi-harmonic FALCON frequencies. All energies are given in $cm^{-1}$.

| No | Type | $\omega$ | 2M | DIF-$f$F2M | | DIFACT-$f$F2M | |
|---|---|---|---|---|---|---|---|
| $f$ | | | | 2 | 3 | 2 | 3 |
| 46 | B2 | 1037.18 | 1067.60 | 1067.86 | 1067.61 | 1067.47 | 1067.45 |
| 47 | B1 | 1129.65 | 1149.35 | 1149.60 | 1149.36 | 1149.03 | 1149.27 |
| 48 | B2 | 1129.70 | 1149.32 | 1149.57 | 1149.34 | 1149.01 | 1149.25 |
| 49 | B2 | 1129.74 | 1121.61 | 1121.66 | 1121.62 | 1121.76 | 1121.64 |
| 50 | B1 | 1129.75 | 1121.56 | 1121.61 | 1121.57 | 1121.71 | 1121.59 |
| 51 | A2 | 1153.00 | 1148.87 | 1148.97 | 1148.87 | 1149.06 | 1148.88 |
| 52 | A1 | 1153.02 | 1148.86 | 1148.97 | 1148.87 | 1149.06 | 1148.88 |
| 53 | B2 | 1159.94 | 1157.54 | 1157.55 | 1157.54 | 1157.45 | 1157.52 |
| 54 | B1 | 1159.94 | 1157.54 | 1157.55 | 1157.54 | 1157.45 | 1157.52 |
| 55 | B1 | 1167.59 | 1175.55 | 1175.15 | 1175.53 | 1175.15 | 1175.52 |
| 56 | B2 | 1167.65 | 1175.55 | 1175.16 | 1175.54 | 1175.15 | 1175.52 |
| 57 | A2 | 1187.06 | 1204.92 | 1204.97 | 1204.91 | 1205.46 | 1205.16 |
| 58 | A1 | 1187.10 | 1204.92 | 1204.96 | 1204.91 | 1205.45 | 1205.16 |
| 59 | A2 | 1189.56 | 1196.93 | 1194.58 | 1196.84 | 1194.45 | 1196.83 |
| 60 | A1 | 1189.57 | 1196.93 | 1194.58 | 1196.84 | 1194.45 | 1196.83 |
| 61 | B1 | 1205.62 | 1224.35 | 1224.46 | 1224.36 | 1224.15 | 1224.22 |
| 62 | B2 | 1205.68 | 1224.35 | 1224.46 | 1224.36 | 1224.15 | 1224.22 |
| 63 | A2 | 1207.05 | 1224.29 | 1224.41 | 1224.29 | 1224.83 | 1224.52 |
| 64 | A1 | 1207.10 | 1224.29 | 1224.41 | 1224.29 | 1224.83 | 1224.52 |
| 65 | B1 | 1224.28 | 1231.22 | 1231.16 | 1231.22 | 1230.92 | 1231.20 |
| 66 | B2 | 1224.31 | 1231.18 | 1231.11 | 1231.18 | 1230.87 | 1231.15 |
| 67 | B1 | 1228.46 | 1242.85 | 1242.85 | 1242.85 | 1242.37 | 1242.73 |
| 68 | B2 | 1228.49 | 1242.89 | 1242.89 | 1242.89 | 1242.41 | 1242.77 |
| 69 | A1 | 1280.44 | 1290.24 | 1289.68 | 1290.23 | 1289.98 | 1290.33 |
| 70 | A2 | 1280.47 | 1290.24 | 1289.68 | 1290.23 | 1289.98 | 1290.33 |
| 71 | A2 | 1304.12 | 1294.93 | 1295.36 | 1294.95 | 1295.31 | 1294.98 |
| 72 | A1 | 1304.13 | 1294.93 | 1295.35 | 1294.95 | 1295.30 | 1294.97 |
| 73 | B1 | 1311.27 | 1303.80 | 1303.96 | 1303.80 | 1303.79 | 1303.79 |
| 74 | B2 | 1311.28 | 1303.80 | 1303.96 | 1303.80 | 1303.79 | 1303.79 |
| 75 | A2 | 1326.27 | 1322.45 | 1322.09 | 1322.44 | 1322.16 | 1322.50 |
| 76 | A1 | 1326.27 | 1322.46 | 1322.09 | 1322.44 | 1322.16 | 1322.50 |
| 77 | B1 | 1334.46 | 1348.85 | 1348.82 | 1348.85 | 1348.43 | 1348.69 |
| 78 | B2 | 1334.47 | 1348.85 | 1348.82 | 1348.84 | 1348.43 | 1348.69 |
| 79 | B1 | 1338.53 | 1348.11 | 1347.89 | 1348.11 | 1347.66 | 1348.01 |
| 80 | B2 | 1338.56 | 1348.11 | 1347.89 | 1348.11 | 1347.66 | 1348.01 |
| 81 | A2 | 1349.58 | 1356.65 | 1355.84 | 1356.63 | 1356.06 | 1356.71 |
| 82 | A1 | 1349.59 | 1356.65 | 1355.84 | 1356.63 | 1356.06 | 1356.71 |
| 83 | A1 | 1482.84 | 1486.46 | 1486.08 | 1486.45 | 1486.39 | 1486.56 |
| 84 | A2 | 1482.85 | 1486.46 | 1486.08 | 1486.45 | 1486.39 | 1486.56 |
| 85 | B1 | 1496.42 | 1500.28 | 1500.08 | 1500.27 | 1499.78 | 1500.16 |
| 86 | B2 | 1496.44 | 1500.28 | 1500.08 | 1500.27 | 1499.79 | 1500.16 |
| 87 | A2 | 1594.75 | 1588.27 | 1587.73 | 1588.25 | 1587.83 | 1588.29 |
| 88 | A1 | 1594.76 | 1588.27 | 1587.73 | 1588.25 | 1587.83 | 1588.29 |
| 89 | B1 | 1649.89 | 1643.71 | 1643.76 | 1643.71 | 1643.57 | 1643.64 |
| 90 | B2 | 1649.89 | 1643.71 | 1643.76 | 1643.71 | 1643.57 | 1643.64 |
| 91 | B1 | 1711.47 | 1704.85 | 1704.96 | 1704.86 | 1704.81 | 1704.80 |
| 92 | B2 | 1711.47 | 1704.85 | 1704.96 | 1704.86 | 1704.81 | 1704.80 |
| 93 | A2 | 1732.04 | 1723.98 | 1724.01 | 1723.98 | 1724.10 | 1724.03 |
| 94 | A1 | 1732.05 | 1723.98 | 1724.01 | 1723.98 | 1724.10 | 1724.03 |
| 95 | A2 | 1816.78 | 1798.56 | 1799.19 | 1798.58 | 1799.12 | 1798.56 |
| 96 | A1 | 1816.79 | 1798.56 | 1799.19 | 1798.57 | 1799.12 | 1798.56 |
| 97 | B1 | 1833.21 | 1815.14 | 1815.42 | 1815.15 | 1815.34 | 1815.15 |
| 98 | B2 | 1833.22 | 1815.14 | 1815.42 | 1815.15 | 1815.34 | 1815.15 |

TABLE S-III continued: Fundamental excitation energies from state-specific VSCF calculations for tetra-phenyl for the different approximations of the potential energy surfaces (all HF-3c). $\omega$ are the corresponding quasi-harmonic FALCON frequencies. All energies are given in $cm^{-1}$.

| No $f$ | Type | $\omega$ | 2M | DIF-$f$F2M 2 | DIF-$f$F2M 3 | DIFACT-$f$F2M 2 | DIFACT-$f$F2M 3 |
|---|---|---|---|---|---|---|---|
| 99 | B1 | 1858.28 | 1840.74 | 1841.12 | 1840.77 | 1841.14 | 1840.75 |
| 100 | B2 | 1858.28 | 1840.74 | 1841.12 | 1840.77 | 1841.14 | 1840.75 |
| 101 | A2 | 1868.41 | 1851.22 | 1852.14 | 1851.26 | 1852.02 | 1851.26 |
| 102 | A1 | 1868.42 | 1851.22 | 1852.14 | 1851.26 | 1852.02 | 1851.26 |
| 103 | B2 | 3689.89 | 3579.94 | 3579.93 | 3579.94 | 3580.32 | 3580.07 |
| 104 | B1 | 3689.89 | 3579.92 | 3579.92 | 3579.93 | 3580.31 | 3580.05 |
| 105 | A2 | 3703.42 | 3591.80 | 3591.42 | 3591.79 | 3591.11 | 3591.65 |
| 106 | A1 | 3703.52 | 3591.80 | 3591.42 | 3591.79 | 3591.10 | 3591.65 |
| 107 | B2 | 3704.48 | 3565.92 | 3565.95 | 3565.92 | 3566.31 | 3566.08 |
| 108 | B1 | 3704.50 | 3565.99 | 3566.02 | 3565.99 | 3566.38 | 3566.15 |
| 109 | B2 | 3711.61 | 3583.04 | 3582.93 | 3583.04 | 3583.47 | 3583.15 |
| 110 | B1 | 3711.64 | 3583.07 | 3582.96 | 3583.07 | 3583.49 | 3583.17 |
| 111 | A2 | 3712.97 | 3600.90 | 3600.51 | 3600.89 | 3600.19 | 3600.75 |
| 112 | A1 | 3713.06 | 3600.91 | 3600.52 | 3600.90 | 3600.21 | 3600.76 |
| 113 | B2 | 3718.76 | 3575.29 | 3575.00 | 3575.28 | 3575.43 | 3575.46 |
| 114 | B1 | 3718.82 | 3575.39 | 3575.10 | 3575.38 | 3575.53 | 3575.56 |
| 115 | A2 | 3721.07 | 3609.11 | 3608.68 | 3609.10 | 3608.37 | 3608.96 |
| 116 | A1 | 3721.21 | 3609.13 | 3608.70 | 3609.12 | 3608.39 | 3608.98 |
| 117 | B2 | 3725.71 | 3631.42 | 3631.36 | 3631.42 | 3631.77 | 3631.58 |
| 118 | B1 | 3725.73 | 3631.40 | 3631.34 | 3631.40 | 3631.75 | 3631.56 |
| 119 | A2 | 3727.74 | 3631.12 | 3630.69 | 3631.10 | 3630.36 | 3630.95 |
| 120 | A1 | 3727.85 | 3631.11 | 3630.69 | 3631.09 | 3630.35 | 3630.94 |

TABLE S-IV: Fundamental excitation energies from state-specific VSCF calculations for hexaphenyl for the different approximations of the potential energy surfaces (all HF-3c). $\omega$ are the corresponding quasi-harmonic FALCON frequencies. All energies are given in $cm^{-1}$. The type labels A1, A2, B1, B2, C1, and C2 refer to intra-fragment vibrations in the respective fragments (see Figure 3 in the main text), IC1 refers to [C1-B1]-(A1)↔(A2)-[B2-C2], IC2 to [C1]-(B1)↔(A1-A2)↔(B2)-[C2], and IC3 to (C1)↔(B1-A1-A2-B2)↔(C2) type of FALCON coordinates (see main text for further explanation).

| No | Type | $\omega$ | 2M | DIF-$f$F2M | | DIFACT-$f$F2M | |
|---|---|---|---|---|---|---|---|
| $f$ | | | | 2 | 3 | 2 | 3 |
| 1 | IC3 | 41.24 | 53.69 | 53.67 | 53.68 | 54.21 | 54.02 |
| 2 | IC3 | 56.88 | 69.30 | 69.42 | 69.29 | 70.31 | 70.59 |
| 3 | IC3 | 59.18 | 102.14 | 102.17 | 102.14 | 103.43 | 106.96 |
| 4 | IC3 | 72.55 | 111.21 | 111.37 | 111.21 | 111.46 | 110.94 |
| 5 | IC3 | 73.99 | 82.70 | 82.48 | 82.70 | 82.93 | 82.50 |
| 6 | IC2 | 83.90 | 115.77 | 116.10 | 115.79 | 119.25 | 119.66 |
| 7 | IC2 | 93.37 | 123.85 | 124.18 | 123.86 | 124.94 | 120.46 |
| 8 | IC3 | 98.34 | 106.53 | 106.23 | 106.52 | 106.84 | 106.76 |
| 9 | IC1 | 102.13 | 129.13 | 129.46 | 129.16 | 130.61 | 128.63 |
| 10 | IC2 | 202.87 | 201.28 | 203.46 | 201.29 | 205.62 | 203.91 |
| 11 | IC2 | 216.07 | 216.30 | 218.47 | 216.32 | 219.55 | 216.44 |
| 12 | IC2 | 288.27 | 289.39 | 288.80 | 289.37 | 288.96 | 289.64 |
| 13 | IC2 | 297.93 | 296.10 | 295.48 | 296.09 | 297.45 | 298.12 |
| 14 | IC1 | 326.16 | 327.22 | 327.91 | 327.22 | 327.50 | 326.46 |
| 15 | IC3 | 335.64 | 338.15 | 338.43 | 338.17 | 339.00 | 337.08 |
| 16 | IC3 | 361.69 | 362.73 | 363.24 | 362.75 | 364.18 | 362.25 |
| 17 | IC1 | 370.76 | 372.93 | 372.25 | 372.89 | 371.43 | 372.43 |
| 18 | IC3 | 376.68 | 372.20 | 372.00 | 372.19 | 372.04 | 372.14 |
| 19 | IC3 | 404.40 | 404.57 | 404.34 | 404.56 | 405.15 | 404.13 |
| 20 | IC2 | 434.15 | 432.89 | 432.32 | 432.90 | 432.38 | 433.32 |
| 21 | IC3 | 447.10 | 446.10 | 445.85 | 446.09 | 446.89 | 445.97 |
| 22 | IC2 | 454.34 | 452.84 | 452.98 | 452.89 | 453.07 | 453.51 |
| 23 | IC3 | 462.35 | 458.54 | 458.36 | 458.54 | 458.38 | 458.77 |
| 24 | C2 | 474.94 | 481.58 | 481.63 | 481.59 | 481.27 | 481.51 |
| 25 | C1 | 474.95 | 481.58 | 481.63 | 481.59 | 481.27 | 481.51 |
| 26 | A2 | 481.49 | 486.20 | 486.38 | 486.18 | 486.51 | 486.45 |
| 27 | A1 | 481.49 | 486.20 | 486.38 | 486.18 | 486.51 | 486.45 |
| 28 | B1 | 481.62 | 486.33 | 486.45 | 486.33 | 487.11 | 486.41 |
| 29 | B2 | 481.63 | 486.33 | 486.45 | 486.33 | 487.11 | 486.41 |
| 30 | IC2 | 483.41 | 482.93 | 482.92 | 482.91 | 482.21 | 482.79 |
| 31 | IC1 | 503.08 | 500.59 | 500.24 | 500.69 | 499.84 | 500.39 |
| 32 | IC2 | 525.04 | 523.62 | 523.46 | 523.62 | 523.32 | 524.09 |
| 33 | IC2 | 536.92 | 531.62 | 530.64 | 531.58 | 530.48 | 529.85 |
| 34 | IC1 | 549.34 | 547.98 | 547.92 | 547.95 | 547.43 | 547.71 |
| 35 | C1 | 566.24 | 574.93 | 575.10 | 574.95 | 574.72 | 574.81 |
| 36 | C2 | 566.24 | 574.93 | 575.10 | 574.95 | 574.72 | 574.81 |
| 37 | IC2 | 600.50 | 595.53 | 594.42 | 595.46 | 594.48 | 595.36 |
| 38 | A1 | 627.63 | 643.02 | 645.44 | 643.07 | 645.62 | 643.35 |
| 39 | A2 | 627.64 | 643.02 | 645.44 | 643.06 | 645.61 | 643.35 |
| 40 | B2 | 628.13 | 643.54 | 645.76 | 643.56 | 646.20 | 643.57 |
| 41 | B1 | 628.15 | 643.53 | 645.76 | 643.56 | 646.20 | 643.57 |
| 42 | IC1 | 658.30 | 652.36 | 650.61 | 652.23 | 650.55 | 653.47 |
| 43 | C1 | 702.97 | 702.53 | 702.56 | 702.53 | 702.41 | 702.43 |

TABLE S-IV continued: Fundamental excitation energies from state-specific VSCF calculations for hexa-phenyl for the different approximations of the potential energy surfaces (all HF-3c). $\omega$ are the corresponding quasi-harmonic FALCON frequencies. All energies are given in $cm^{-1}$.

| No | Type | $\omega$ | 2M | DIF-$f$F2M | | DIFACT-$f$F2M | |
|---|---|---|---|---|---|---|---|
| $f$ | | | | 2 | 3 | 2 | 3 |
| 44 | C2 | 702.98 | 702.53 | 702.56 | 702.53 | 702.41 | 702.43 |
| 45 | A1 | 719.86 | 717.14 | 717.07 | 717.13 | 717.07 | 717.16 |
| 46 | A2 | 719.87 | 717.14 | 717.07 | 717.13 | 717.07 | 717.16 |
| 47 | B2 | 719.92 | 717.17 | 717.12 | 717.17 | 717.25 | 717.20 |
| 48 | B1 | 719.93 | 717.17 | 717.12 | 717.17 | 717.24 | 717.20 |
| 49 | C2 | 782.58 | 782.21 | 782.30 | 782.21 | 782.08 | 782.06 |
| 50 | C1 | 782.59 | 782.20 | 782.29 | 782.21 | 782.08 | 782.06 |
| 51 | C1 | 838.69 | 856.85 | 857.05 | 856.87 | 856.49 | 856.67 |
| 52 | C2 | 838.70 | 856.84 | 857.04 | 856.86 | 856.48 | 856.66 |
| 53 | B1 | 859.82 | 857.40 | 857.28 | 857.39 | 857.41 | 857.40 |
| 54 | B2 | 859.82 | 857.40 | 857.28 | 857.39 | 857.42 | 857.40 |
| 55 | A2 | 859.87 | 857.56 | 857.43 | 857.53 | 857.44 | 857.54 |
| 56 | A1 | 859.87 | 857.56 | 857.43 | 857.53 | 857.44 | 857.54 |
| 57 | A1 | 884.37 | 879.96 | 879.36 | 879.97 | 879.45 | 880.15 |
| 58 | A2 | 884.38 | 879.96 | 879.36 | 879.97 | 879.45 | 880.14 |
| 59 | B2 | 884.63 | 880.18 | 879.54 | 880.19 | 879.85 | 880.21 |
| 60 | B1 | 884.64 | 880.18 | 879.54 | 880.19 | 879.85 | 880.21 |
| 61 | C1 | 913.91 | 937.57 | 937.63 | 937.57 | 937.04 | 937.37 |
| 62 | C2 | 913.93 | 937.58 | 937.64 | 937.58 | 937.05 | 937.38 |
| 63 | A1 | 1019.59 | 1044.48 | 1045.62 | 1044.51 | 1045.87 | 1044.89 |
| 64 | A2 | 1019.64 | 1044.48 | 1045.62 | 1044.51 | 1045.87 | 1044.89 |
| 65 | B2 | 1019.88 | 1044.87 | 1045.85 | 1044.89 | 1046.37 | 1044.87 |
| 66 | B1 | 1019.92 | 1044.87 | 1045.85 | 1044.89 | 1046.38 | 1044.87 |
| 67 | A1 | 1032.64 | 1062.19 | 1062.88 | 1062.22 | 1063.15 | 1062.64 |
| 68 | A2 | 1032.70 | 1062.19 | 1062.88 | 1062.22 | 1063.15 | 1062.64 |
| 69 | B2 | 1033.06 | 1062.82 | 1063.30 | 1062.85 | 1063.85 | 1062.81 |
| 70 | B1 | 1033.11 | 1062.82 | 1063.30 | 1062.85 | 1063.85 | 1062.82 |
| 71 | C1 | 1037.13 | 1068.29 | 1068.56 | 1068.31 | 1068.21 | 1068.11 |
| 72 | C2 | 1037.18 | 1068.29 | 1068.56 | 1068.31 | 1068.21 | 1068.11 |
| 73 | C1 | 1129.68 | 1149.65 | 1149.89 | 1149.65 | 1149.27 | 1149.45 |
| 74 | C2 | 1129.70 | 1149.58 | 1149.82 | 1149.58 | 1149.20 | 1149.38 |
| 75 | C1 | 1129.75 | 1121.81 | 1121.88 | 1121.82 | 1121.98 | 1121.83 |
| 76 | C2 | 1129.75 | 1121.95 | 1122.02 | 1121.96 | 1122.12 | 1121.98 |
| 77 | A1 | 1152.85 | 1148.73 | 1148.93 | 1148.74 | 1148.92 | 1148.74 |
| 78 | A2 | 1152.86 | 1148.73 | 1148.93 | 1148.74 | 1148.92 | 1148.74 |
| 79 | B2 | 1153.00 | 1148.77 | 1148.89 | 1148.78 | 1149.05 | 1148.83 |
| 80 | B1 | 1153.01 | 1148.77 | 1148.89 | 1148.78 | 1149.05 | 1148.83 |
| 81 | C1 | 1159.94 | 1157.50 | 1157.52 | 1157.51 | 1157.40 | 1157.46 |
| 82 | C2 | 1159.95 | 1157.50 | 1157.52 | 1157.51 | 1157.40 | 1157.46 |
| 83 | C1 | 1167.65 | 1176.32 | 1175.99 | 1176.30 | 1176.00 | 1176.16 |
| 84 | C2 | 1167.68 | 1176.32 | 1176.00 | 1176.31 | 1176.00 | 1176.16 |
| 85 | A1 | 1186.92 | 1205.18 | 1205.34 | 1205.18 | 1205.55 | 1205.54 |
| 86 | A2 | 1186.96 | 1205.18 | 1205.34 | 1205.18 | 1205.55 | 1205.54 |
| 87 | B2 | 1187.03 | 1205.52 | 1205.58 | 1205.52 | 1206.07 | 1205.50 |
| 88 | B1 | 1187.06 | 1205.52 | 1205.58 | 1205.52 | 1206.07 | 1205.50 |
| 89 | B2 | 1189.67 | 1198.16 | 1195.83 | 1198.04 | 1195.55 | 1197.86 |
| 90 | B1 | 1189.70 | 1198.15 | 1195.82 | 1198.03 | 1195.54 | 1197.85 |
| 91 | A1 | 1190.58 | 1198.72 | 1195.59 | 1198.50 | 1195.60 | 1198.45 |
| 92 | A2 | 1190.61 | 1198.73 | 1195.59 | 1198.50 | 1195.61 | 1198.45 |
| 93 | C1 | 1205.63 | 1224.87 | 1224.99 | 1224.88 | 1224.71 | 1224.72 |
| 94 | C2 | 1205.66 | 1224.87 | 1224.99 | 1224.88 | 1224.71 | 1224.72 |
| 95 | A1 | 1206.85 | 1224.50 | 1224.74 | 1224.50 | 1224.95 | 1224.84 |
| 96 | A2 | 1206.89 | 1224.50 | 1224.74 | 1224.50 | 1224.95 | 1224.84 |

TABLE S-IV continued: Fundamental excitation energies from state-specific VSCF calculations for hexa-phenyl for the different approximations of the potential energy surfaces (all HF-3c). $\omega$ are the corresponding quasi-harmonic FALCON frequencies. All energies are given in $cm^{-1}$.

| No | Type | $\omega$ | 2M | DIF-$f$F2M | | DIFACT-$f$F2M | |
|---|---|---|---|---|---|---|---|
| $f$ | | | | 2 | 3 | 2 | 3 |
| 97 | B2 | 1207.01 | 1224.89 | 1225.02 | 1224.89 | 1225.40 | 1224.85 |
| 98 | B1 | 1207.05 | 1224.89 | 1225.02 | 1224.89 | 1225.40 | 1224.85 |
| 99 | C1 | 1224.31 | 1231.56 | 1231.51 | 1231.55 | 1231.22 | 1231.42 |
| 100 | C2 | 1224.31 | 1231.54 | 1231.50 | 1231.54 | 1231.20 | 1231.40 |
| 101 | C1 | 1228.46 | 1243.32 | 1243.33 | 1243.32 | 1242.81 | 1243.09 |
| 102 | C2 | 1228.48 | 1243.34 | 1243.35 | 1243.33 | 1242.83 | 1243.11 |
| 103 | B2 | 1280.46 | 1290.54 | 1289.97 | 1290.52 | 1290.38 | 1290.62 |
| 104 | B1 | 1280.47 | 1290.54 | 1289.97 | 1290.52 | 1290.38 | 1290.62 |
| 105 | A1 | 1280.78 | 1290.72 | 1289.96 | 1290.70 | 1289.98 | 1290.78 |
| 106 | A2 | 1280.79 | 1290.72 | 1289.96 | 1290.70 | 1289.98 | 1290.78 |
| 107 | A1 | 1303.87 | 1295.73 | 1296.26 | 1295.78 | 1296.29 | 1295.77 |
| 108 | A2 | 1303.87 | 1295.73 | 1296.26 | 1295.78 | 1296.29 | 1295.77 |
| 109 | B2 | 1304.07 | 1295.66 | 1296.17 | 1295.70 | 1296.12 | 1295.58 |
| 110 | B1 | 1304.08 | 1295.66 | 1296.16 | 1295.69 | 1296.12 | 1295.58 |
| 111 | C2 | 1311.26 | 1304.62 | 1304.87 | 1304.64 | 1304.71 | 1304.44 |
| 112 | C2 | 1311.28 | 1304.62 | 1304.87 | 1304.64 | 1304.71 | 1304.44 |
| 113 | B2 | 1326.20 | 1322.75 | 1322.43 | 1322.74 | 1322.54 | 1322.74 |
| 114 | B1 | 1326.21 | 1322.75 | 1322.42 | 1322.73 | 1322.54 | 1322.74 |
| 115 | A1 | 1326.26 | 1322.97 | 1322.48 | 1322.94 | 1322.50 | 1322.97 |
| 116 | A2 | 1326.27 | 1322.97 | 1322.48 | 1322.94 | 1322.50 | 1322.97 |
| 117 | C1 | 1334.43 | 1349.09 | 1349.09 | 1349.09 | 1348.64 | 1348.81 |
| 118 | C2 | 1334.43 | 1349.09 | 1349.08 | 1349.09 | 1348.64 | 1348.80 |
| 119 | C2 | 1338.48 | 1348.14 | 1347.92 | 1348.13 | 1347.65 | 1348.00 |
| 120 | C1 | 1338.49 | 1348.13 | 1347.92 | 1348.13 | 1347.65 | 1348.00 |
| 121 | B1 | 1349.59 | 1356.85 | 1356.02 | 1356.81 | 1356.31 | 1356.90 |
| 122 | B2 | 1349.60 | 1356.85 | 1356.02 | 1356.81 | 1356.32 | 1356.90 |
| 123 | A1 | 1349.95 | 1357.02 | 1355.87 | 1356.96 | 1355.87 | 1357.02 |
| 124 | A2 | 1349.95 | 1357.02 | 1355.87 | 1356.96 | 1355.87 | 1357.02 |
| 125 | B1 | 1482.80 | 1486.41 | 1486.02 | 1486.39 | 1486.47 | 1486.54 |
| 126 | B2 | 1482.82 | 1486.41 | 1486.02 | 1486.39 | 1486.47 | 1486.54 |
| 127 | A1 | 1482.95 | 1486.54 | 1485.98 | 1486.51 | 1485.99 | 1486.61 |
| 128 | A2 | 1482.96 | 1486.53 | 1485.98 | 1486.51 | 1485.99 | 1486.60 |
| 129 | C2 | 1496.43 | 1500.36 | 1500.17 | 1500.35 | 1499.82 | 1500.17 |
| 130 | C1 | 1496.45 | 1500.36 | 1500.16 | 1500.35 | 1499.82 | 1500.17 |
| 131 | B1 | 1594.74 | 1588.73 | 1588.23 | 1588.71 | 1588.37 | 1588.70 |
| 132 | B2 | 1594.76 | 1588.73 | 1588.23 | 1588.71 | 1588.37 | 1588.71 |
| 133 | A2 | 1594.80 | 1588.79 | 1588.09 | 1588.75 | 1588.10 | 1588.76 |
| 134 | A1 | 1594.81 | 1588.79 | 1588.09 | 1588.75 | 1588.10 | 1588.76 |
| 135 | C1 | 1649.92 | 1644.09 | 1644.20 | 1644.11 | 1643.98 | 1643.92 |
| 136 | C2 | 1649.93 | 1644.09 | 1644.20 | 1644.11 | 1643.98 | 1643.91 |
| 137 | C2 | 1711.42 | 1704.95 | 1705.08 | 1704.97 | 1704.92 | 1704.85 |
| 138 | C1 | 1711.43 | 1704.95 | 1705.08 | 1704.97 | 1704.92 | 1704.85 |
| 139 | A2 | 1731.83 | 1724.06 | 1724.20 | 1724.07 | 1724.22 | 1724.09 |
| 140 | A1 | 1731.83 | 1724.06 | 1724.20 | 1724.07 | 1724.22 | 1724.09 |
| 141 | B2 | 1731.96 | 1724.02 | 1724.09 | 1724.03 | 1724.21 | 1724.08 |
| 142 | B1 | 1731.97 | 1724.01 | 1724.09 | 1724.03 | 1724.21 | 1724.07 |
| 143 | A1 | 1816.47 | 1798.88 | 1799.74 | 1798.92 | 1799.76 | 1798.86 |
| 144 | A2 | 1816.48 | 1798.88 | 1799.74 | 1798.92 | 1799.76 | 1798.86 |
| 145 | B2 | 1816.74 | 1799.15 | 1799.85 | 1799.19 | 1799.73 | 1799.10 |
| 146 | B1 | 1816.79 | 1799.15 | 1799.84 | 1799.18 | 1799.73 | 1799.10 |
| 147 | C2 | 1833.20 | 1815.55 | 1815.87 | 1815.57 | 1815.79 | 1815.44 |
| 148 | C1 | 1833.21 | 1815.55 | 1815.87 | 1815.57 | 1815.78 | 1815.44 |
| 149 | C1 | 1858.28 | 1841.15 | 1841.58 | 1841.19 | 1841.62 | 1841.10 |

TABLE S-IV continued: Fundamental excitation energies from state-specific VSCF calculations for hexa-phenyl for the different approximations of the potential energy surfaces (all HF-3c). $\omega$ are the corresponding quasi-harmonic FALCON frequencies. All energies are given in $cm^{-1}$.

| No | Type | $\omega$ | 2M | DIF-$f$F2M | | DIFACT-$f$F2M | |
|---|---|---|---|---|---|---|---|
| $f$ | | | | 2 | 3 | 2 | 3 |
| 150 | C1 | 1858.29 | 1841.15 | 1841.58 | 1841.19 | 1841.62 | 1841.10 |
| 151 | A1 | 1867.84 | 1851.34 | 1852.61 | 1851.45 | 1852.61 | 1851.42 |
| 152 | A2 | 1867.84 | 1851.34 | 1852.61 | 1851.45 | 1852.61 | 1851.42 |
| 153 | B1 | 1868.35 | 1851.74 | 1852.73 | 1851.81 | 1852.55 | 1851.71 |
| 154 | B2 | 1868.36 | 1851.74 | 1852.73 | 1851.81 | 1852.55 | 1851.71 |
| 155 | C1 | 3689.88 | 3579.90 | 3579.92 | 3579.92 | 3580.35 | 3580.12 |
| 156 | C2 | 3689.89 | 3579.88 | 3579.90 | 3579.90 | 3580.32 | 3580.09 |
| 157 | B1 | 3703.47 | 3591.83 | 3591.47 | 3591.82 | 3591.08 | 3591.77 |
| 158 | B2 | 3703.47 | 3591.84 | 3591.47 | 3591.82 | 3591.08 | 3591.77 |
| 159 | A2 | 3703.68 | 3592.06 | 3591.48 | 3592.03 | 3591.43 | 3591.84 |
| 160 | A1 | 3703.68 | 3592.07 | 3591.48 | 3592.03 | 3591.43 | 3591.85 |
| 161 | C1 | 3704.45 | 3565.84 | 3565.90 | 3565.86 | 3566.27 | 3566.07 |
| 162 | C2 | 3704.46 | 3565.81 | 3565.86 | 3565.83 | 3566.24 | 3566.04 |
| 163 | C1 | 3711.61 | 3582.86 | 3582.78 | 3582.88 | 3583.41 | 3583.11 |
| 164 | C2 | 3711.63 | 3582.91 | 3582.84 | 3582.93 | 3583.46 | 3583.16 |
| 165 | B1 | 3713.01 | 3600.85 | 3600.48 | 3600.84 | 3600.10 | 3600.79 |
| 166 | B2 | 3713.01 | 3600.88 | 3600.51 | 3600.86 | 3600.12 | 3600.81 |
| 167 | A2 | 3713.22 | 3601.17 | 3600.59 | 3601.14 | 3600.54 | 3600.95 |
| 168 | A1 | 3713.22 | 3601.18 | 3600.59 | 3601.14 | 3600.54 | 3600.96 |
| 169 | C1 | 3718.71 | 3575.30 | 3575.04 | 3575.30 | 3575.50 | 3575.54 |
| 170 | C2 | 3718.76 | 3575.27 | 3575.00 | 3575.26 | 3575.46 | 3575.50 |
| 171 | B2 | 3721.11 | 3609.11 | 3608.69 | 3609.09 | 3608.32 | 3609.04 |
| 172 | B1 | 3721.13 | 3609.08 | 3608.66 | 3609.06 | 3608.29 | 3609.01 |
| 173 | A1 | 3721.32 | 3609.43 | 3608.79 | 3609.39 | 3608.74 | 3609.20 |
| 174 | A2 | 3721.33 | 3609.43 | 3608.79 | 3609.39 | 3608.74 | 3609.20 |
| 175 | C1 | 3725.67 | 3631.37 | 3631.34 | 3631.39 | 3631.78 | 3631.61 |
| 176 | C2 | 3725.70 | 3631.34 | 3631.30 | 3631.35 | 3631.74 | 3631.58 |
| 177 | B2 | 3727.80 | 3631.12 | 3630.71 | 3631.10 | 3630.31 | 3631.04 |
| 178 | B1 | 3727.80 | 3631.12 | 3630.71 | 3631.10 | 3630.31 | 3631.05 |
| 179 | A2 | 3727.99 | 3631.36 | 3630.78 | 3631.31 | 3630.73 | 3631.11 |
| 180 | A1 | 3727.99 | 3631.36 | 3630.78 | 3631.31 | 3630.72 | 3631.11 |

TABLE S-V: Fundamental excitation energies ($\Delta E$) from state-specific VSCF calculations for tetra-phenyl for DIF-2F2M representation of the potential energy surface (RI-BP86/SVP). $\omega$ are the corresponding quasi-harmonic FALCON frequencies. All energies are given in $cm^{-1}$. The type labels A1, A2, B1, and B2 refer to intra-fragment vibrations in the respective fragments (see Figure 3 in the main text), IC1 refers to [B1]-(A1)↔(A2)-[B2] and IC2 to (B1)↔(A1-A2)↔(B2) type of FALCON coordinate (see main text for further explanation).

| No | Type | $\omega$ | $\Delta E$ |
|---|---|---|---|
| 1 | IC2 | 39.41 | 54.03 |
| 2 | IC2 | 47.33 | 91.91 |
| 3 | IC2 | 62.27 | 71.89 |
| 4 | IC2 | 66.90 | 103.26 |
| 5 | IC2 | 76.05 | 89.27 |
| 6 | IC1 | 81.26 | 113.42 |
| 7 | IC2 | 111.62 | 118.66 |
| 8 | IC1 | 276.55 | 275.97 |
| 9 | IC2 | 297.12 | 298.53 |
| 10 | IC1 | 321.06 | 319.67 |
| 11 | IC2 | 331.53 | 326.39 |
| 12 | IC2 | 341.62 | 341.21 |
| 13 | IC2 | 376.16 | 374.59 |
| 14 | B2 | 405.06 | 410.58 |
| 15 | B1 | 405.14 | 410.70 |
| 16 | A2 | 408.76 | 413.55 |
| 17 | A1 | 408.84 | 413.32 |
| 18 | IC1 | 424.32 | 419.44 |
| 19 | IC2 | 439.44 | 436.11 |
| 20 | IC2 | 470.48 | 463.38 |
| 21 | IC1 | 482.98 | 479.29 |
| 22 | B2 | 483.30 | 489.66 |
| 23 | B1 | 483.39 | 489.89 |
| 24 | A2 | 532.22 | 548.10 |
| 25 | A1 | 532.52 | 547.87 |
| 26 | IC1 | 579.81 | 570.01 |
| 27 | B1 | 610.95 | 607.15 |
| 28 | B2 | 611.00 | 607.14 |
| 29 | A1 | 624.15 | 618.34 |
| 30 | A2 | 624.20 | 618.46 |
| 31 | B2 | 681.56 | 677.55 |
| 32 | B1 | 681.58 | 677.71 |
| 33 | B2 | 696.96 | 715.26 |
| 34 | B1 | 697.08 | 715.57 |
| 35 | A1 | 736.49 | 724.12 |
| 36 | A2 | 736.49 | 724.23 |
| 37 | A2 | 749.93 | 745.43 |
| 38 | A1 | 750.04 | 745.05 |
| 39 | B1 | 752.37 | 759.12 |
| 40 | B2 | 752.61 | 759.18 |
| 41 | A2 | 823.44 | 845.08 |
| 42 | A1 | 823.98 | 844.83 |
| 43 | A2 | 828.30 | 843.35 |
| 44 | A1 | 828.58 | 843.08 |
| 45 | B2 | 830.61 | 852.04 |
| 46 | B1 | 830.73 | 852.37 |

TABLE S-V continued: Fundamental excitation energies ($\Delta E$) from state-specific VSCF calculations for tetra-phenyl for DIF-2F2M representation of the potential energy surface (RI-BP86/SVP). $\omega$ are the corresponding quasi-harmonic FALCON frequencies. All energies are given in $cm^{-1}$.

| No. | Type | $\omega$ | $\Delta E$ |
|---|---|---|---|
| 47 | B1 | 904.42 | 912.86 |
| 48 | B2 | 904.53 | 912.64 |
| 49 | A2 | 952.83 | 956.62 |
| 50 | A1 | 953.02 | 956.23 |
| 51 | A2 | 961.15 | 967.71 |
| 52 | A1 | 961.45 | 967.32 |
| 53 | B1 | 961.83 | 968.90 |
| 54 | B2 | 961.88 | 968.73 |
| 55 | B2 | 981.93 | 970.64 |
| 56 | B1 | 981.99 | 970.67 |
| 57 | B1 | 984.53 | 986.52 |
| 58 | B2 | 984.61 | 986.44 |
| 59 | A2 | 993.53 | 984.90 |
| 60 | A1 | 993.72 | 984.70 |
| 61 | B1 | 1023.59 | 1015.58 |
| 62 | B2 | 1023.74 | 1015.53 |
| 63 | B1 | 1071.05 | 1065.07 |
| 64 | B2 | 1071.62 | 1065.10 |
| 65 | A2 | 1103.54 | 1099.26 |
| 66 | A1 | 1103.54 | 1098.62 |
| 67 | A2 | 1127.39 | 1117.31 |
| 68 | A1 | 1127.79 | 1117.07 |
| 69 | B2 | 1130.20 | 1116.99 |
| 70 | B1 | 1130.37 | 1117.40 |
| 71 | B1 | 1137.65 | 1134.37 |
| 72 | B2 | 1137.80 | 1134.30 |
| 73 | A2 | 1139.82 | 1127.63 |
| 74 | A1 | 1140.12 | 1127.19 |
| 75 | B1 | 1160.13 | 1152.96 |
| 76 | B2 | 1160.57 | 1153.02 |
| 77 | A1 | 1172.47 | 1162.87 |
| 78 | A2 | 1172.49 | 1163.45 |
| 79 | A2 | 1268.48 | 1254.24 |
| 80 | A1 | 1268.88 | 1253.77 |
| 81 | B1 | 1280.23 | 1265.15 |
| 82 | B2 | 1280.66 | 1265.09 |
| 83 | A2 | 1324.98 | 1304.98 |
| 84 | A1 | 1325.04 | 1304.87 |
| 85 | B1 | 1358.86 | 1339.09 |
| 86 | B2 | 1359.05 | 1338.99 |
| 87 | A2 | 1406.58 | 1385.09 |
| 88 | A1 | 1406.66 | 1384.56 |
| 89 | B1 | 1428.80 | 1408.61 |
| 90 | B2 | 1429.00 | 1408.56 |
| 91 | B1 | 1473.32 | 1452.89 |
| 92 | B2 | 1473.52 | 1452.77 |
| 93 | A2 | 1482.35 | 1462.13 |
| 94 | A1 | 1482.53 | 1461.66 |
| 95 | A2 | 1549.38 | 1526.15 |
| 96 | A1 | 1549.55 | 1525.80 |
| 97 | B1 | 1582.16 | 1556.26 |
| 98 | B2 | 1582.19 | 1556.11 |
| 99 | B1 | 1610.54 | 1585.81 |
| 100 | B2 | 1610.64 | 1585.67 |

TABLE S-V continued: Fundamental excitation energies ($\Delta E$) from state-specific VSCF calculations for tetra-phenyl for DIF-2F2M representation of the potential energy surface (RI-BP86/SVP). $\omega$ are the corresponding quasi-harmonic FALCON frequencies. All energies are given in $cm^{-1}$.

| No. | Type | $\omega$ | $\Delta E$ |
|---|---|---|---|
| 101 | A2 | 1615.13 | 1591.59 |
| 102 | A1 | 1615.28 | 1591.19 |
| 103 | B2 | 3099.20 | 2962.45 |
| 104 | B1 | 3099.25 | 2963.46 |
| 105 | A2 | 3103.95 | 2962.17 |
| 106 | A1 | 3104.04 | 2962.54 |
| 107 | B1 | 3104.87 | 2960.37 |
| 108 | A2 | 3105.08 | 2962.84 |
| 109 | B2 | 3105.09 | 2960.63 |
| 110 | A1 | 3105.14 | 2963.29 |
| 111 | B1 | 3113.37 | 2952.18 |
| 112 | B2 | 3113.58 | 2950.81 |
| 113 | A2 | 3118.35 | 2978.11 |
| 114 | B1 | 3118.37 | 2975.42 |
| 115 | A1 | 3118.45 | 2977.77 |
| 116 | B2 | 3118.55 | 2975.24 |
| 117 | A2 | 3120.68 | 3005.83 |
| 118 | A1 | 3120.76 | 3005.46 |
| 119 | B2 | 3126.49 | 3009.22 |
| 120 | B1 | 3126.64 | 3007.97 |
